# Supplementary material for: Absolutely continuous spectrum for the Anderson model on a product of a tree with a finite graph
Source: arXiv:1008.2949 source file (2011-10-28)
Supplement: Supplementary file 1 [file appendix1.tex]

\beginsection
\hd{Appendix 1}

\beginproofof{\thmrf{imwt}}

(i) It is enough to prove this statement for $\Gamma$ of the form $\Gamma = \twovec{I&B}{0&I}$ with $B^T=B$, $\Gamma = \twovec{0&-I}{I&0}$ or $\Gamma = \twovec{A&0}{0&{A^T}^{-1}}$, since these generate ${\rm Sp}(4,\RR)$.
If $\Gamma=\twovec{I&B}{0&I}$ with $B^T=B$ then $\Gamma\cdot (X+iY) = (X + B) + iY$. So $Z_1-Z_2$, $Y_1$ and $Y_2$ are invariant under the action of $\Gamma$ which implies that $w_{p}(Z_1,Z_2) = \|Y_2^{-1/2}(Z_1-Z_2)^*Y_1^{-1}(Z_1-Z_2)Y_2^{-1/2}\|_{1+p}^{1+p}$ is invariant too.
If $\Gamma=\twovec{0&-I}{I&0}$ then $\Gamma\cdot Z = -Z^{-1}$. The invariance of $w_p$ follows from the identities $-Z_1^{-1}+Z_2^{-1}=Z_1^{-1}(Z_1-Z_2)Z_2^{-1}$ and $\Im Z_i^{-1} = Z_i^{-1}Y_i{Z_i^*}^{-1}$,
together with the fact that $\|C^* C\|_{1+p} = \|C C^*\|_{1+p}$. The proof for the case $\Gamma = \twovec{A&0}{0&{A^T}^{-1}}$ is similar.

(ii) Since $t>0$ we have $(Y+t)^{-1} \le Y^{-1}$. Thus the required inequality follows from
$$\displaylines{\quad
\|(Y_2+t)^{-1/2}(Z_1-Z_2)^*(Y_1+t)^{-1}(Z_1-Z_2)(Y_2+t)^{-1/2}\|_{1+p}^{1+p}
\hfill\cr\hfill
\eqalign{
&\le \|(Y_2+t)^{-1/2}(Z_1-Z_2)^*Y_1^{-1}(Z_1-Z_2)(Y_2+t)^{-1/2}\|_{1+p}^{1+p}\cr
&= \|Y_1^{-1/2}(Z_1-Z_2)(Y_2+t)^{-1}(Z_1-Z_2)^*Y_1^{-1/2}\|_{1+p}^{1+p}\cr
&\le \|Y_1^{-1/2}(Z_1-Z_2)Y_2^{-1}(Z_1-Z_2)^*Y_1^{-1/2}\|_{1+p}^{1+p}\cr
&=\|Y_2^{-1/2}(Z_1-Z_2)^*Y_1^{-1}(Z_1-Z_2)Y_2^{-1/2}\|_{1+p}^{1+p}.\cr
}\quad}$$

(iii) We follow [FHS3]. For $\lambda\in R_\epsilon$, $Y_\lambda$ is bounded above and below by positive constants. Thus, $\Im G = \Yh_\lambda\Im Z\,\Yh_\lambda < C \Im Z$ with constants uniform in $\lambda$. Since all norms are equivalent for $2\times 2$ matrices, and by the convexity of $|\cdot|^{1+p}$, it suffices to show that for $Z=X+iY$,   $\|Y\|_1 \le \|(Z-iI)^*Y^{-1}(Z-iI)\|_1 + 4$. Because $Y$ is positive definite,
\be{imy}\eqalign{
\|Y\|_1 &= \tr(Y)\cr
&\le \tr(Y+Y^{-1}-2I) + 4\cr
&= \tr((Y-I)Y^{-1}(Y-I)) + 4\cr
&\le \tr((Y-I)Y^{-1}(Y-I) + XY^{-1}X) + 4\cr
&= \tr((X-i(Y-I))Y^{-1}(X+i(Y-I))) + 4\cr
&=\|(Z-iI)^*Y^{-1}(Z-iI)\|_1 + 4.\cr
}\ee
This completes the proof. For future reference, notice that \rf{imy} also holds with $\|Y^{-1}\|_1$ on the left side.

(iv) Using $\|AB\|_{1+p}\le\|A\|_{2(1+p)}\|B\|_{2(1+p)}$ and $\|A\|_{2(1+p)}^2 = \|A^* A\|_{1+p}$, together with the comment following \rf{imy} we find that for any $\epsilon>0$
$$\displaylines{
\|(Z+ Q-iI)^*Y^{-1}(Z+Q-iI)\|_{1+p} 
\hfill\cr\hfill
\eqalign{
&\le \|(Z-iI)^*Y^{-1}(Z-iI)\|_{1+p} 
+ 2 \|Q\Ymh\|_{2(1+p)}\|\Ymh (Z-iI)\|_{2(1+p)} + \|(QY^{-1}Q\|_{1+p}\cr
&\le (1+\epsilon)\|(Z-iI)^*Y^{-1}(Z-iI)\|_{1+p} + (1+1/\epsilon)\|Q\|^{2}\|Y^{-1}\|_{1+p}\cr
&\le (1+\epsilon + C_\epsilon\|Q\|^{2})\|(Z-iI)^*Y^{-1}(Z-iI)\|_{1+p} + C_\epsilon\|Q\|^{2}.\cr
}\quad}$$
Now the result follows from the fact that for any $\epsilon>0$, there is $C_\epsilon$ such that
$|a + b|^{1+p} \le (1+\epsilon)|a|^{1+p} + C_\epsilon|b|^{1+p}$ for positive $a$ and $b$.

\endproofof

\beginlemmalabel{isthisobvious}
Let $Z = X + i Y$ be a complex $n\times n$ matrix with $X$ and $Y$ real and symmetric. Moreover assume that $Y \geq t_1 > 0$.
Then $Z$ is bijective and $\| Z^{-1} \| \leq t_1^{-1}$. 
\endlemmalabel

\beginproof
For all  $\varphi \in \CC^n$,
$$
 t_1  \| \varphi \|^2 \leq ( \varphi , Y \varphi)  = {\rm Im} ( \varphi , Z \varphi ) \leq | (\varphi , Z \varphi ) | \leq \| \varphi \| \| Z \varphi \| , 
$$
and hence 
\be{eq:lastlemmainappendix}
\| \varphi \| \leq t_1^{-1} \| Z  \varphi \|       .
\ee
This implies that $Z$ is injective and hence bijective since $n$ is finite.
Inserting $\varphi = Z^{-1} \psi$ into  \rf{eq:lastlemmainappendix}, we find
$$
\| Z^{-1} \psi \| \leq t_1^{-1} \| \psi \| 
$$
for all $\psi \in \CC^n$. This yields the claim.
\endproof

\endsection
